# Supplementary material for: Probably Approximately Optimal Query Optimization
Source: arXiv:1511.01782 source file (2015-11-05)
Supplement: Supplementary file 1 [file appendix.tex]

%\newpage

%\clearpage

\appendix

For completeness, we provide additional experimental results for queries with star-shaped join graphs. Figures~\ref{FigIterSmallStar} and \ref{FigCallSmallStar} show a comparison between different region extension algorithms for small star queries joining five tables. Figures~\ref{FigIterBigStar} and \ref{FigCallBigStar} show results for star queries joining ten tables. The results are consistent with the ones for chain queries and show that slope-based extensions pay off by reducing the number of iterations, optimizer calls, and required samples at the same time.

\regionFiguresPack{5-table star}{Small}{Star}

\regionFiguresPack{10-table star}{Big}{Star}

Figures~\ref{FigSampleIterSmallStar} to \ref{FigSampleCallsSmallStar} compare different sampling strategies for small star queries. Figures~\ref{FigSampleIterBigStar} to \ref{FigSampleCallsBigStar} report the analogue results for larger queries. Again the results are consistent with the ones for chain queries.

\samplingFiguresPack{5-table star}{Small}{Star}{}

\samplingFiguresPack{10-table star}{Big}{Star}{}

Uniform sampling usually minimizes the number of required samples while it has the maximal number of iterations and optimizer invocations. The exponential sampling schemes reduce the number of iterations and optimizer calls significantly while causing a moderate overhead in terms of additional samples. Adaptive sampling has usually the lowest number of iterations and optimizer calls while it often requires the largest number of samples. This changes once the number of predicates becomes elevated (at least four) where adaptive sampling starts requiring fewer samples than the exponential sampling strategy. This shows the advantage of distributing samples non-uniformly over different predicates.

%\balance
